# Supplementary material for: Quantifying Dynamic Tilting in Halide Perovskites: Chemical Trends and Local Correlations
Source: arXiv:2304.07402 ancillary file (2023-04-14)
Supplement: Supplementary file 1 [file supplemental-material.pdf]

**Supplemental Material:**

# Quantifying Dynamic Tilting in Halide Perovskites: Chemical Trends and Local Correlations

Julia Wiktor[1,*], Erik Fransson[1], Dominik Kubicki[2], and Paul Erhart[1,*]

[1] *Department of Physics, Chalmers University of Technology, SE-41296, Gothenburg, Sweden*
[2]*School of Chemistry, University of Birmingham, Birmingham, UK*
[*]*julia.wiktor@chalmers.se, erhart@chalmers.se*

# Contents

**Supplemental Figures** **2**

**Supplemental Tables** **5**

# Supplemental Figures

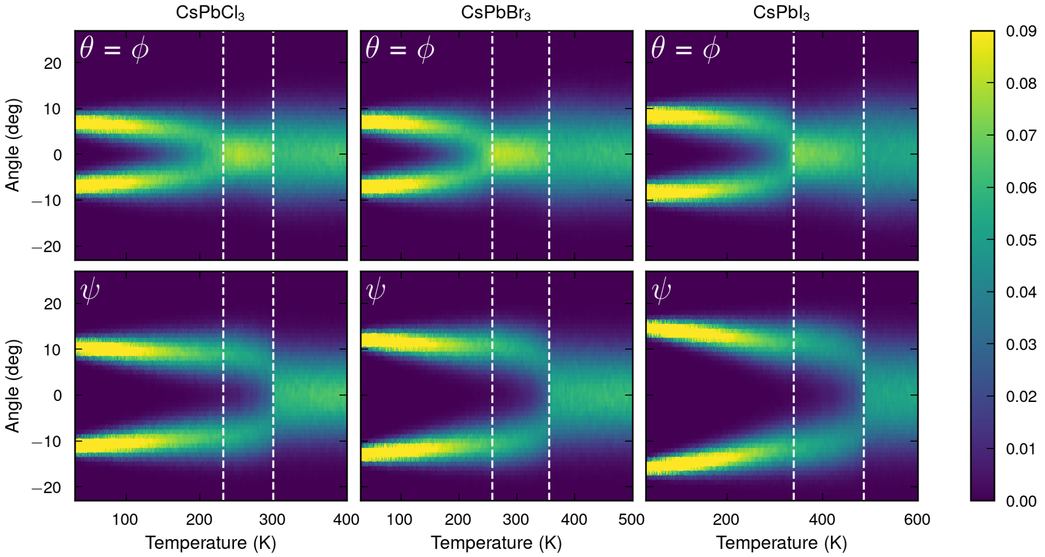


Figure S1: Maps of tilt angles as a function of temperature in $CsPbCl_3$, $CsPbBr_3$, and $CsPbI_3$ from models based on the vdW-DF-cx functional. Dashed vertical lines indicate the orthorhombic-to-tetragonal and tetragonal-to-cubic phase transitions.

[!htbp]

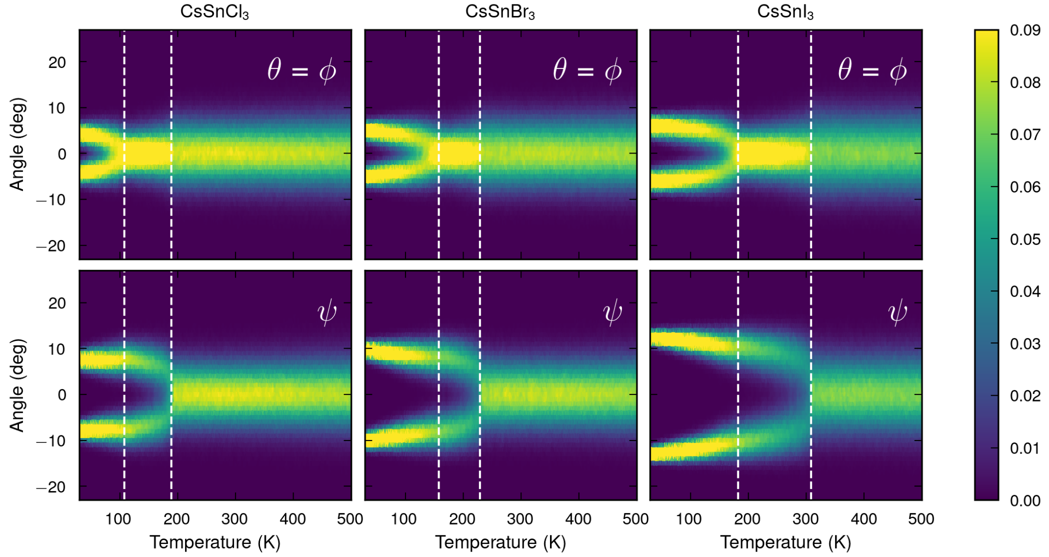


Figure S2: Maps of tilt angles as a function of temperature in $CsSnCl_3$, $CsSnBr_3$, and $CsSnI_3$ from models based on the vdW-DF-cx functional. Dashed vertical lines indicate the orthorhombic-to-tetragonal and tetragonal-to-cubic phase transitions.

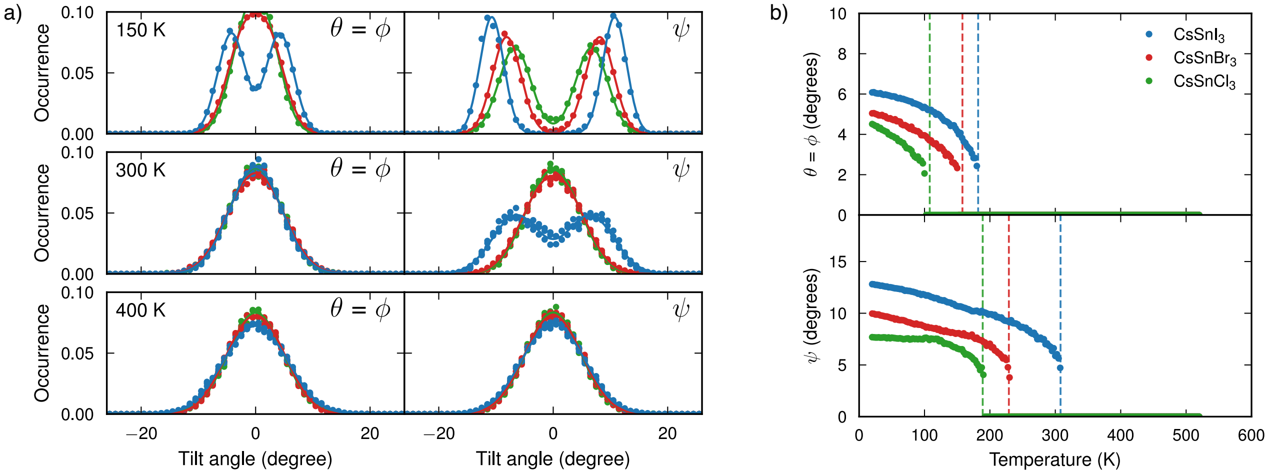


Figure S3: (a) Probability distribution of octahedral tilts at 150, 300, and 400 K in $CsSnCl_3$, $CsSnBr_3$, and $CsSnI_3$, as described by the three Euler angles $\theta$, $\phi$, and $\psi$. (b) Position of the maximum in the tilt angle distribution as extracted from double Gaussian fits. Vertical dashed lines indicate phase transitions.

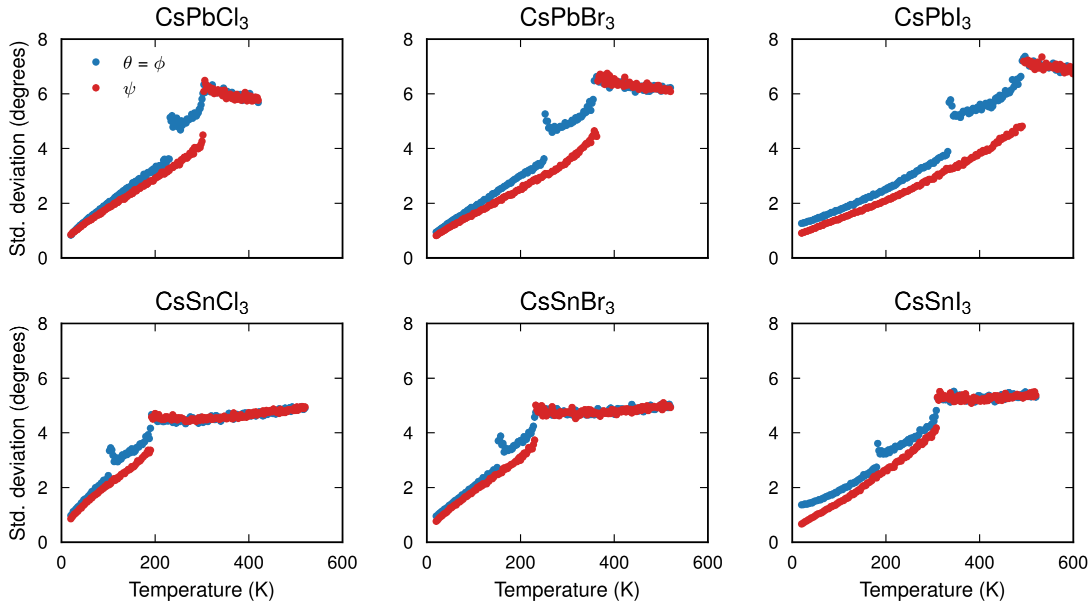


Figure S4: Standard deviation $\sigma$ of the tilt angle distributions as extracted from double Gaussian fits.

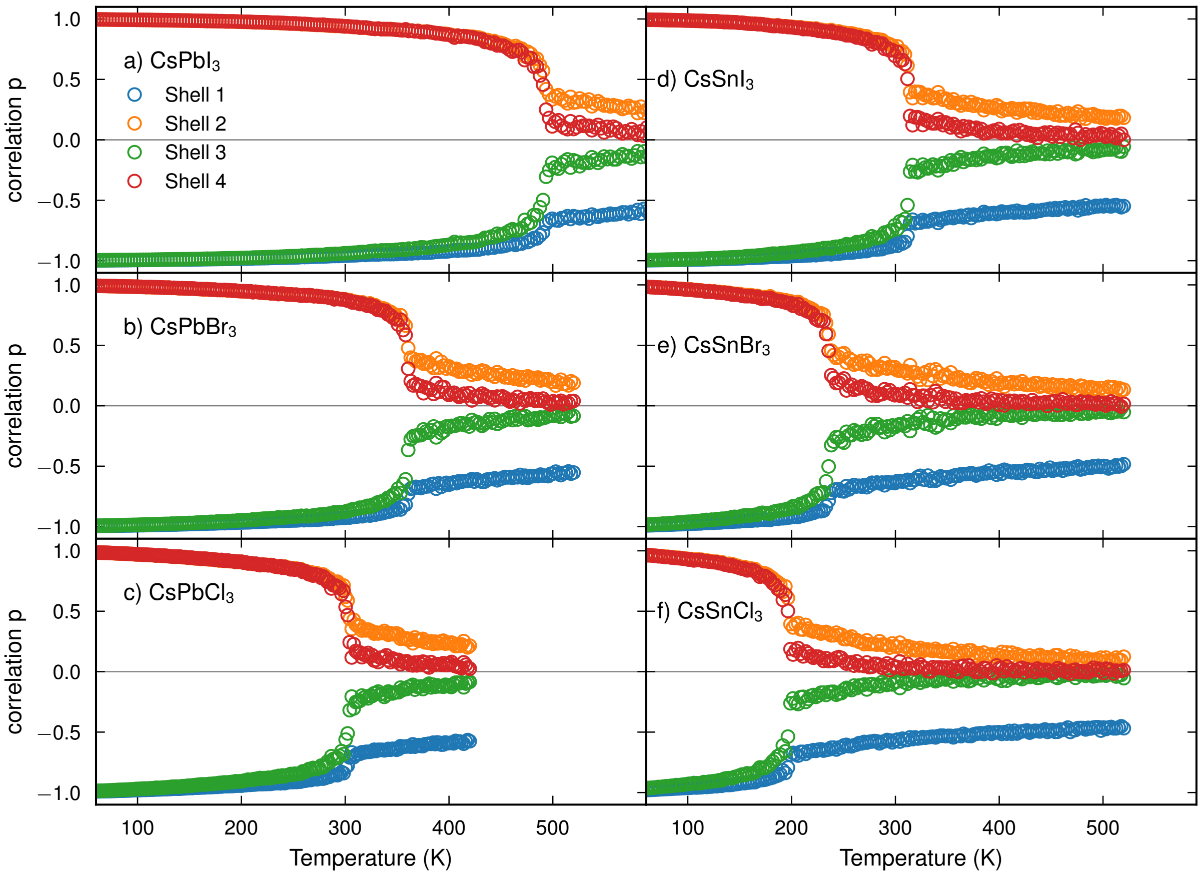


Figure S5: The correlation $p$ of tilt-angles around the $z$-axis calculated along heating simulation for the neighbor shells along the [100] direction.

# Supplemental Tables

Table S1: Overview of data used for training NEP models. $N_{\text{structures}}$: Number of structures. $N_{\text{atoms}}$: Total number of atoms. RMSE: root mean squared error in units of meV atom$^{-1}$, meV Å$^{-1}$, and meV atom$^{-1}$ for energy, forces, and virials, respectively.

| Material | XC | $N_{\text{structures}}$ | $N_{\text{atoms}}$ | Energy | | Forces | | Virials | |
|---|---|---|---|---|---|---|---|---|---|
| | | | | $R^2$ | RMSE | $R^2$ | RMSE | $R^2$ | RMSE |
| $CsPbCl_3$ | vdW-DF-cx | 633 | 65 820 | 0.99984 | 1.2 | 0.98833 | 46.4 | 0.99955 | 13.0 |
| $CsPbBr_3$ | vdW-DF-cx | 618 | 63 255 | 0.99985 | 1.1 | 0.98676 | 45.1 | 0.99968 | 11.1 |
| $CsPbI_3$ | vdW-DF-cx | 674 | 65 060 | 0.99966 | 1.8 | 0.98623 | 47.5 | 0.99945 | 14.5 |
| $CsPbI_3$ | PBE | 510 | 45 800 | 0.99990 | 1.0 | 0.98620 | 43.1 | 0.99960 | 12.6 |
| $CsPbI_3$ | PBEsol | 697 | 69 340 | 0.99975 | 1.9 | 0.99093 | 50.6 | 0.99955 | 15.2 |
| $CsPbI_3$ | SCAN | 657 | 61 360 | 0.99976 | 2.1 | 0.98714 | 51.4 | 0.99962 | 16.0 |
| $CsSnCl_3$ | vdW-DF-cx | 751 | 72 085 | 0.99974 | 1.5 | 0.98401 | 58.1 | 0.99922 | 16.7 |
| $CsSnBr_3$ | vdW-DF-cx | 785 | 77 500 | 0.99976 | 1.6 | 0.98331 | 54.6 | 0.99914 | 18.5 |
| $CsSnI_3$ | vdW-DF-cx | 778 | 77 420 | 0.99941 | 2.5 | 0.98010 | 55.5 | 0.99884 | 21.9 |

Table S2: Atomic shells treated among the valence electrons in the projector augmented wave setups used in the VASP DFT calculations with.

| Element | Valence configuration |
|---|---|
| Cs | $5s^2 5p^6 6s^1$ |
| Sn | $5s^2 5p^2$ |
| Pb | $6s^2 6p^2$ |
| Cl | $3s^2 3p^5$ |
| Br | $4s^2 4p^5$ |
| I | $5s^2 5p^5$ |

Table S3: Phase transition temperatures in K found for different halide perovskites using the vdW-DF-cx functional. Values were extracted from the temperature dependence of heat capacity.

| | ortho-tetra | tetra-cubic |
|---|---|---|
| $CsPbCl_3$ | 232 | 300 |
| $CsPbBr_3$ | 258 | 356 |
| $CsPbI_3$ | 340 | 487 |
| $CsSnCl_3$ | 108 | 189 |
| $CsSnBr_3$ | 158 | 229 |
| $CsSnI_3$ | 182 | 308 |
